# Supplementary material for: UADB: Unsupervised Anomaly Detection Booster
Source: arXiv:2306.01997 source file (2023-12-26)
Supplement: Supplementary file 1 [file appendix.tex]

\begin{table*}
\scriptsize
\centering
\setlength{\tabcolsep}{1.6mm}{
\begin{tabular}{c|c|cccccccccc|c} 
\toprule
\multirow{2}{*}{\diagbox{\textbf{Dataset}}{\textbf{Performance}}} & \textbf{Teacher} & \multicolumn{10}{c|}{\textbf{Student with multiple iterations}}                                                                                                                                             & \textbf{\textbf{Improvement}}         \\ 
\cmidrule{2-13}
                                                                  & \textbf{IForest} & \textbf{Iter 1} & \textbf{Iter 2} & \textbf{Iter~3} & \textbf{Iter~4} & \textbf{Iter~5} & \textbf{sIter~6} & \textbf{Iter~7} & \textbf{Iter~8} & \textbf{Iter~9} & \textbf{Iter 10} & \textbf{(Iter 10) - Teacher}  \\ 
\midrule
\textbf{speech}                                                   & 0.5057           & 0.5828          & 0.5790           & 0.5926          & 0.6002          & 0.6093          & 0.6130            & 0.6174          & 0.6200            & 0.6194          & 0.6233           & 0.1176                                \\ 
\midrule
\textbf{Wilt}                                                     & 0.4276           & 0.5921          & 0.4407          & 0.5073          & 0.4989          & 0.5153          & 0.5305           & 0.5312          & 0.5309          & 0.5367          & 0.5364           & 0.1088                                \\ 
\midrule
\textbf{satellite}                                                & 0.6668           & 0.6835          & 0.6988          & 0.7060           & 0.7117          & 0.7179          & 0.7250            & 0.7327          & 0.7413          & 0.7511          & 0.7625           & 0.0957                                \\ 
\midrule
\textbf{vowels}                                                   & 0.8118           & 0.7988          & 0.8318          & 0.8441          & 0.8488          & 0.8617          & 0.8707           & 0.8826          & 0.8918          & 0.9026          & 0.9066           & 0.0949                                \\ 
\midrule
\textbf{abalone}                                                  & 0.4989           & 0.5337          & 0.5435          & 0.5481          & 0.5524          & 0.5569          & 0.5589           & 0.5601          & 0.5603          & 0.5647          & 0.5663           & 0.0674                                \\ 
\midrule
\textbf{SpamBase}                                                 & 0.5997           & 0.6325          & 0.6333          & 0.6369          & 0.6393          & 0.6417          & 0.6433           & 0.6454          & 0.6461          & 0.6465          & 0.6472           & 0.0475                                \\ 
\midrule
\textbf{skin}                                                     & 0.6756           & 0.6433          & 0.6705          & 0.6683          & 0.6970           & 0.6992          & 0.7032           & 0.7137          & 0.7127          & 0.7132          & 0.7216           & 0.0459                                \\ 
\midrule
\textbf{landsat}                                                  & 0.4716           & 0.4570           & 0.4677          & 0.4786          & 0.4854          & 0.4905          & 0.4962           & 0.5035          & 0.5089          & 0.5148          & 0.5172           & 0.0457                                \\ 
\midrule
\textbf{nternetAds}                                               & 0.6988           & 0.7021          & 0.705           & 0.707           & 0.7088          & 0.7113          & 0.715            & 0.7193          & 0.7243          & 0.7292          & 0.7348           & 0.0359                                \\ 
\midrule
\textbf{agnews\_1}                                                & 0.5995           & 0.6226          & 0.6258          & 0.6287          & 0.6272          & 0.6295          & 0.6305           & 0.6312          & 0.6324          & 0.6320           & 0.6327           & 0.0332                                \\
\bottomrule
\end{tabular}}
\end{table*}

\begin{table*}
    \scriptsize
    \centering
    \caption{Caption here}
    \begin{subtable}[t]{0.495\linewidth}
        \caption{AUCROC}
        \setlength{\tabcolsep}{0.8mm}{
        \begin{tabular}{c|c|ccccc|c} 
            \toprule
                                 & \textbf{Teacher} & \multicolumn{5}{c|}{\textbf{Student with multiple iterations}}                                    & \multicolumn{1}{l}{\textbf{Improvement}}  \\ 
            \midrule
            \textbf{Datasets}    & \textbf{IForest} & \textbf{iter\textit{ }2} & \textbf{iter 4} & \textbf{iter 6} & \textbf{iter 8} & \textbf{iter 10} & \textbf{Improvement}                      \\ 
            \midrule
            \textbf{speech}      & 0.5057           & 0.5790                   & 0.6002          & 0.6130          & 0.6200          & 0.6233           & 0.1176                                    \\
            \textbf{Wilt}        & 0.4276           & 0.4407                   & 0.4989          & 0.5305          & 0.5309          & 0.5364           & 0.1088                                    \\
            \textbf{satellite}   & 0.6668           & 0.6988                   & 0.7117          & 0.7250          & 0.7413          & 0.7625           & 0.0957                                    \\
            \textbf{vowels}      & 0.8118           & 0.8318                   & 0.8488          & 0.8707          & 0.8918          & 0.9066           & 0.0949                                    \\
            \textbf{abalone}     & 0.4989           & 0.5435                   & 0.5524          & 0.5589          & 0.5603          & 0.5663           & 0.0674                                    \\
            \textbf{SpamBase}    & 0.5997           & 0.6333                   & 0.6393          & 0.6433          & 0.6461          & 0.6472           & 0.0475                                    \\
            \textbf{skin}        & 0.6756           & 0.6705                   & 0.6970           & 0.7032          & 0.7127          & 0.7216           & 0.0459                                    \\
            \textbf{landsat}     & 0.4716           & 0.4677                   & 0.4854          & 0.4962          & 0.5089          & 0.5172           & 0.0457                                    \\
            \textbf{~~~~InternetAds~~~~} & 0.6988           & 0.7050                   & 0.7088          & 0.7150          & 0.7243          & 0.7348           & 0.0359                                    \\
            \textbf{agnews\_1}   & 0.5995           & 0.6258                   & 0.6272          & 0.6305          & 0.6324          & 0.6327           & 0.0332                                    \\
            \bottomrule
        \end{tabular}}
    \end{subtable}
    \begin{subtable}[t]{0.495\linewidth}
        \caption{AP}
        \setlength{\tabcolsep}{0.8mm}{
        \begin{tabular}{c|c|ccccc|c} 
            \toprule
                                     & \textbf{Teacher} & \multicolumn{5}{c|}{\textbf{Student with multiple iterations }}                                                   & \textbf{Improvement}  \\ 
            \midrule
            \textbf{Dataset}         & \textbf{IForest} & \textbf{iter 2} & \textbf{iter 4} & \textbf{iter 6} & \textbf{iter 8} & \textbf{iter 10} & \textbf{Improvement}  \\ 
            \midrule
            \textbf{pendigits}   & 0.3392           & 0.3995          & 0.4154          & 0.4505          & 0.4973          & 0.5524           & 0.2132                \\
            \textbf{vowels}      & 0.1825           & 0.1743          & 0.1835          & 0.2463          & 0.3143          & 0.3408           & 0.1582                \\
            \textbf{satellite}   & 0.6248           & 0.7074          & 0.7163          & 0.7252          & 0.7317          & 0.7399           & 0.1151                \\
            \textbf{~~~~InternetAds~~~~} & 0.5078           & 0.5166          & 0.5221          & 0.5313          & 0.5468          & 0.5588           & 0.0510                 \\
            \textbf{abalone}      & 0.5111           & 0.531           & 0.5379          & 0.5443          & 0.5468          & 0.5529           & 0.0418                \\
            \textbf{wine}        & 0.1905           & 0.2051          & 0.2141          & 0.2244          & 0.2281          & 0.228            & 0.0376                \\
            \textbf{Hepatitis}   & 0.2534           & 0.2702          & 0.2893          & 0.2931          & 0.2924          & 0.2892           & 0.0358                \\
            \textbf{cardio}       & 0.4841           & 0.5010           & 0.5083          & 0.5071          & 0.5125          & 0.5153           & 0.0312                \\
            \textbf{skin}        & 0.2619           & 0.2597          & 0.2760           & 0.2801          & 0.2864          & 0.2925           & 0.0306                \\
            \textbf{Stamps}      & 0.3182           & 0.3379          & 0.3457          & 0.3510           & 0.3486          & 0.3468           & 0.0286                \\
            \bottomrule
        \end{tabular}}
    \end{subtable}
    
    \begin{subtable}[t]{0.495\linewidth}
        \caption{AUCROC}
        \setlength{\tabcolsep}{0.8mm}{
        \begin{tabular}{c|c|ccccc|c} 
            \toprule
                                         & \textbf{Teacher} & \multicolumn{5}{c|}{\textbf{Student with multiple iterations }}                                                                       & \textbf{Improvement}  \\ 
            \midrule
            \textbf{Dataset}             & \textbf{LOF}     & \textbf{iter 2} & \textbf{iter 4} & \textbf{iter 6} & \textbf{iter 8} & \textbf{iter 10} & \textbf{Improvement}  \\ 
            \midrule
            \textbf{http}            & 0.3685           & 1                        & 1                        & 1                        & 1                        & 1                         & 0.6315                \\
            \textbf{shuttle}         & 0.4886           & 0.9199                   & 0.9244                   & 0.9691                   & 0.9537                   & 0.9525                    & 0.4638                \\
            \textbf{satimage-2}      & 0.4702           & 0.5677                   & 0.6909                   & 0.7618                   & 0.8402                   & 0.9146                    & 0.4444                \\
            \textbf{optdigits}       & 0.5819           & 0.8488                   & 0.8884                   & 0.9128                   & 0.9318                   & 0.9438                    & 0.3619                \\
            \textbf{musk}            & 0.4586           & 0.5008                   & 0.5584                   & 0.6137                   & 0.6848                   & 0.7528                    & 0.2942                \\
            \textbf{satellite}       & 0.5523           & 0.7405                   & 0.7655                   & 0.7749                   & 0.7868                   & 0.7902                    & 0.238                 \\
            \textbf{speech}          & 0.5035           & 0.6552                   & 0.6823                   & 0.7019                   & 0.7115                   & 0.7182                    & 0.2147                \\
            \textbf{FashionMNIST\_5} & 0.6806           & 0.7116                   & 0.7807                   & 0.8211                   & 0.8572                   & 0.8847                    & 0.2041                \\
            \textbf{FashionMNIST\_1} & 0.6669           & 0.7405                   & 0.7768                   & 0.8083                   & 0.833                    & 0.8566                    & 0.1897                \\
            \textbf{landsat}         & 0.5436           & 0.704                    & 0.7161                   & 0.713                    & 0.713                    & 0.7096                    & 0.166                 \\
            \bottomrule
            \end{tabular}}
    \end{subtable}
    \begin{subtable}[t]{0.495\linewidth}
        \caption{AP}
        \setlength{\tabcolsep}{0.8mm}{
        \begin{tabular}{c|c|ccccc|c} 
            \toprule
                                     & \textbf{Teacher} & \multicolumn{5}{c|}{\textbf{Student with multiple iterations }}                          & \textbf{Improvement}  \\ 
            \midrule
            \textbf{Dataset}         & \textbf{LOF}     & \textbf{iter 2} & \textbf{iter~4} & \textbf{iter~6} & \textbf{iter~8} & \textbf{iter~10} & \textbf{improvement}  \\ 
            \midrule
            \textbf{http}            & 0.0603           & 1               & 1               & 1               & 1               & 1                & 0.9397                \\
            \textbf{shuttle}         & 0.0958           & 0.6814          & 0.7598          & 0.873           & 0.7902          & 0.7882           & 0.6924                \\
            \textbf{optdigits}       & 0.0732           & 0.1114          & 0.1825          & 0.2627          & 0.3593          & 0.4551           & 0.3819                \\
            \textbf{satellite}       & 0.3746           & 0.6268          & 0.675           & 0.6887          & 0.7047          & 0.7117           & 0.3371                \\
            \textbf{WDBC}            & 0.1026           & 0.1757          & 0.2627          & 0.3202          & 0.3604          & 0.3754           & 0.2727                \\
            \textbf{FashionMNIST\_7} & 0.2485           & 0.3013          & 0.3345          & 0.3796          & 0.4325          & 0.4875           & 0.239                 \\
            \textbf{FashionMNIST\_1} & 0.1679           & 0.213           & 0.2372          & 0.2771          & 0.3291          & 0.3943           & 0.2263                \\
            \textbf{FashionMNIST\_8} & 0.1246           & 0.1602          & 0.1917          & 0.2374          & 0.2996          & 0.3365           & 0.2119                \\
            \textbf{FashionMNIST\_5} & 0.1936           & 0.2157          & 0.2422          & 0.2776          & 0.3292          & 0.3971           & 0.2035                \\
            \textbf{smtp}            & 0.0526           & 0.0556          & 0.3333          & 0.3333          & 0.25            & 0.25             & 0.1974                \\
            \bottomrule
            \end{tabular}}
    \end{subtable}
    
    \begin{subtable}[t]{0.495\linewidth}
        \caption{AUCROC}
        \setlength{\tabcolsep}{1.2mm}{
        \begin{tabular}{c|c|ccccc|c} 
            \toprule
                                 & \textbf{Teacher} & \multicolumn{5}{c|}{\textbf{Student with multiple iterations}}                                    & \multicolumn{1}{l}{\textbf{Improvement}}  \\ 
            \midrule
            \textbf{Datasets}    & \textbf{IForest} & \textbf{iter\textit{ }2} & \textbf{iter 4} & \textbf{iter 6} & \textbf{iter 8} & \textbf{iter 10} & \textbf{Improvement}                      \\ 
            \midrule
            \textbf{speech}      & 0.5057           & 0.5790                   & 0.6002          & 0.6130          & 0.6200          & 0.6233           & 0.1176                                    \\
            \textbf{Wilt}        & 0.4276           & 0.4407                   & 0.4989          & 0.5305          & 0.5309          & 0.5364           & 0.1088                                    \\
            \textbf{satellite}   & 0.6668           & 0.6988                   & 0.7117          & 0.7250          & 0.7413          & 0.7625           & 0.0957                                    \\
            \textbf{vowels}      & 0.8118           & 0.8318                   & 0.8488          & 0.8707          & 0.8918          & 0.9066           & 0.0949                                    \\
            \textbf{abalone}     & 0.4989           & 0.5435                   & 0.5524          & 0.5589          & 0.5603          & 0.5663           & 0.0674                                    \\
            \textbf{SpamBase}    & 0.5997           & 0.6333                   & 0.6393          & 0.6433          & 0.6461          & 0.6472           & 0.0475                                    \\
            \textbf{skin}        & 0.6756           & 0.6705                   & 0.6970           & 0.7032          & 0.7127          & 0.7216           & 0.0459                                    \\
            \textbf{landsat}     & 0.4716           & 0.4677                   & 0.4854          & 0.4962          & 0.5089          & 0.5172           & 0.0457                                    \\
            \textbf{InternetAds} & 0.6988           & 0.7050                   & 0.7088          & 0.7150          & 0.7243          & 0.7348           & 0.0359                                    \\
            \textbf{agnews\_1}   & 0.5995           & 0.6258                   & 0.6272          & 0.6305          & 0.6324          & 0.6327           & 0.0332                                    \\
            \bottomrule
        \end{tabular}}
    \end{subtable}
    \begin{subtable}[t]{0.495\linewidth}
        \caption{AP}
        \setlength{\tabcolsep}{1.2mm}{
        \begin{tabular}{c|c|ccccc|c} 
            \toprule
                                     & \textbf{Teacher} & \multicolumn{5}{c|}{\textbf{Student with multiple iterations }}                                                   & \textbf{Improvement}  \\ 
            \midrule
            \textbf{Dataset}         & \textbf{IForest} & \textbf{iter 2} & \textbf{iter 4} & \textbf{iter 6} & \textbf{iter 8} & \textbf{iter 10} & \textbf{Improvement}  \\ 
            \midrule
            \textbf{pendigits}   & 0.3392           & 0.3995          & 0.4154          & 0.4505          & 0.4973          & 0.5524           & 0.2132                \\
            \textbf{vowels}      & 0.1825           & 0.1743          & 0.1835          & 0.2463          & 0.3143          & 0.3408           & 0.1582                \\
            \textbf{satellite}   & 0.6248           & 0.7074          & 0.7163          & 0.7252          & 0.7317          & 0.7399           & 0.1151                \\
            \textbf{InternetAds} & 0.5078           & 0.5166          & 0.5221          & 0.5313          & 0.5468          & 0.5588           & 0.0510                 \\
            \textbf{abalone}      & 0.5111           & 0.531           & 0.5379          & 0.5443          & 0.5468          & 0.5529           & 0.0418                \\
            \textbf{wine}        & 0.1905           & 0.2051          & 0.2141          & 0.2244          & 0.2281          & 0.228            & 0.0376                \\
            \textbf{Hepatitis}   & 0.2534           & 0.2702          & 0.2893          & 0.2931          & 0.2924          & 0.2892           & 0.0358                \\
            \textbf{cardio}       & 0.4841           & 0.5010           & 0.5083          & 0.5071          & 0.5125          & 0.5153           & 0.0312                \\
            \textbf{skin}        & 0.2619           & 0.2597          & 0.2760           & 0.2801          & 0.2864          & 0.2925           & 0.0306                \\
            \textbf{Stamps}      & 0.3182           & 0.3379          & 0.3457          & 0.3510           & 0.3486          & 0.3468           & 0.0286                \\
            \bottomrule
        \end{tabular}}
    \end{subtable}
    
    \begin{subtable}[t]{0.495\linewidth}
        \caption{AUCROC}
        \setlength{\tabcolsep}{1.2mm}{
        \begin{tabular}{c|c|ccccc|c} 
            \toprule
                                 & \textbf{Teacher} & \multicolumn{5}{c|}{\textbf{Student with multiple iterations}}                                    & \multicolumn{1}{l}{\textbf{Improvement}}  \\ 
            \midrule
            \textbf{Datasets}    & \textbf{IForest} & \textbf{iter\textit{ }2} & \textbf{iter 4} & \textbf{iter 6} & \textbf{iter 8} & \textbf{iter 10} & \textbf{Improvement}                      \\ 
            \midrule
            \textbf{speech}      & 0.5057           & 0.5790                   & 0.6002          & 0.6130          & 0.6200          & 0.6233           & 0.1176                                    \\
            \textbf{Wilt}        & 0.4276           & 0.4407                   & 0.4989          & 0.5305          & 0.5309          & 0.5364           & 0.1088                                    \\
            \textbf{satellite}   & 0.6668           & 0.6988                   & 0.7117          & 0.7250          & 0.7413          & 0.7625           & 0.0957                                    \\
            \textbf{vowels}      & 0.8118           & 0.8318                   & 0.8488          & 0.8707          & 0.8918          & 0.9066           & 0.0949                                    \\
            \textbf{abalone}     & 0.4989           & 0.5435                   & 0.5524          & 0.5589          & 0.5603          & 0.5663           & 0.0674                                    \\
            \textbf{SpamBase}    & 0.5997           & 0.6333                   & 0.6393          & 0.6433          & 0.6461          & 0.6472           & 0.0475                                    \\
            \textbf{skin}        & 0.6756           & 0.6705                   & 0.6970           & 0.7032          & 0.7127          & 0.7216           & 0.0459                                    \\
            \textbf{landsat}     & 0.4716           & 0.4677                   & 0.4854          & 0.4962          & 0.5089          & 0.5172           & 0.0457                                    \\
            \textbf{InternetAds} & 0.6988           & 0.7050                   & 0.7088          & 0.7150          & 0.7243          & 0.7348           & 0.0359                                    \\
            \textbf{agnews\_1}   & 0.5995           & 0.6258                   & 0.6272          & 0.6305          & 0.6324          & 0.6327           & 0.0332                                    \\
            \bottomrule
        \end{tabular}}
    \end{subtable}
    \begin{subtable}[t]{0.495\linewidth}
        \caption{AP}
        \setlength{\tabcolsep}{1.2mm}{
        \begin{tabular}{c|c|ccccc|c} 
            \toprule
                                     & \textbf{Teacher} & \multicolumn{5}{c|}{\textbf{Student with multiple iterations }}                                                   & \textbf{Improvement}  \\ 
            \midrule
            \textbf{Dataset}         & \textbf{IForest} & \textbf{iter 2} & \textbf{iter 4} & \textbf{iter 6} & \textbf{iter 8} & \textbf{iter 10} & \textbf{Improvement}  \\ 
            \midrule
            \textbf{pendigits}   & 0.3392           & 0.3995          & 0.4154          & 0.4505          & 0.4973          & 0.5524           & 0.2132                \\
            \textbf{vowels}      & 0.1825           & 0.1743          & 0.1835          & 0.2463          & 0.3143          & 0.3408           & 0.1582                \\
            \textbf{satellite}   & 0.6248           & 0.7074          & 0.7163          & 0.7252          & 0.7317          & 0.7399           & 0.1151                \\
            \textbf{InternetAds} & 0.5078           & 0.5166          & 0.5221          & 0.5313          & 0.5468          & 0.5588           & 0.0510                 \\
            \textbf{abalone}      & 0.5111           & 0.531           & 0.5379          & 0.5443          & 0.5468          & 0.5529           & 0.0418                \\
            \textbf{wine}        & 0.1905           & 0.2051          & 0.2141          & 0.2244          & 0.2281          & 0.228            & 0.0376                \\
            \textbf{Hepatitis}   & 0.2534           & 0.2702          & 0.2893          & 0.2931          & 0.2924          & 0.2892           & 0.0358                \\
            \textbf{cardio}       & 0.4841           & 0.5010           & 0.5083          & 0.5071          & 0.5125          & 0.5153           & 0.0312                \\
            \textbf{skin}        & 0.2619           & 0.2597          & 0.2760           & 0.2801          & 0.2864          & 0.2925           & 0.0306                \\
            \textbf{Stamps}      & 0.3182           & 0.3379          & 0.3457          & 0.3510           & 0.3486          & 0.3468           & 0.0286                \\
            \bottomrule
        \end{tabular}}
    \end{subtable}
    \label{tab:array}
\end{table*}

\begin{table*}
\scriptsize
\centering
\caption{\method's performance on some representative unsupervised AD methods (teacher) in terms of AUCROC and AP.
For each method, we show the results of the best 10 datasets among over 80 datasets.
Here, the total iterations of cascade student is set to 10.
}
\setlength{\tabcolsep}{0.8mm}{
\begin{tabular}{c|cccccc|ccc|cccccc|c} 
\cmidrule[\heavyrulewidth]{1-8}\cmidrule[\heavyrulewidth]{10-17}
\multicolumn{8}{c}{\textbf{Student's improvement compared to Teacher (IForest) in terms of AUCROC}}                                                                                       &                      & \multicolumn{8}{c}{\textbf{ Student's improvement compared to Teacher (IForest) in terms of AP}}                                                                                           \\ 
\cmidrule{1-8}\cmidrule{10-17}
\textbf{Datasets}        & \textbf{Teacher}     & \textbf{iter 2}      & \textbf{iter 4}      & \textbf{iter~6}      & \textbf{iter~8}      & \textbf{iter~10}     & \textbf{Improvement} &                      & \textbf{Datasets}        & \textbf{Teacher}     & \textbf{iter~2}      & \textbf{iter~4}      & \textbf{iter~6}      & \textbf{iter~8}      & \textbf{iter~10}     & \textbf{Improvement}  \\ 
\cmidrule{1-8}\cmidrule{10-17}
\textbf{speech}          & 0.5057               & 0.579                & 0.6002               & 0.613                & 0.62                 & 0.6233               & 0.1176               &                      & \textbf{pendigits}       & 0.3392               & 0.3995               & 0.4154               & 0.4505               & 0.4973               & 0.5524               & 0.2132                \\ 
\cline{1-8}\cline{10-17}
\textbf{Wilt}            & 0.4276               & 0.4407               & 0.4989               & 0.5305               & 0.5309               & 0.5364               & 0.1088               &                      & \textbf{vowels}          & 0.1825               & 0.1743               & 0.1835               & 0.2463               & 0.3143               & 0.3408               & 0.1582                \\ 
\cline{1-8}\cline{10-17}
\textbf{satellite}       & 0.6668               & 0.6988               & 0.7117               & 0.725                & 0.7413               & 0.7625               & 0.0957               &                      & \textbf{satellite}       & 0.6248               & 0.7074               & 0.7163               & 0.7252               & 0.7317               & 0.7399               & 0.1151                \\ 
\cline{1-8}\cline{10-17}
\textbf{vowels}          & 0.8118               & 0.8318               & 0.8488               & 0.8707               & 0.8918               & 0.9066               & 0.0949               &                      & \textbf{InternetAds}     & 0.5078               & 0.5166               & 0.5221               & 0.5313               & 0.5468               & 0.5588               & 0.051                 \\ 
\cline{1-8}\cline{10-17}
\textbf{abalone}         & 0.4989               & 0.5435               & 0.5524               & 0.5589               & 0.5603               & 0.5663               & 0.0674               &                      & \textbf{abalone}         & 0.5111               & 0.531                & 0.5379               & 0.5443               & 0.5468               & 0.5529               & 0.0418                \\ 
\cline{1-8}\cline{10-17}
\textbf{SpamBase}        & 0.5997               & 0.6333               & 0.6393               & 0.6433               & 0.6461               & 0.6472               & 0.0475               &                      & \textbf{wine}            & 0.1905               & 0.2051               & 0.2141               & 0.2244               & 0.2281               & 0.228                & 0.0376                \\ 
\cline{1-8}\cline{10-17}
\textbf{skin}            & 0.6756               & 0.6705               & 0.697                & 0.7032               & 0.7127               & 0.7216               & 0.0459               &                      & \textbf{Hepatitis}       & 0.2534               & 0.2702               & 0.2893               & 0.2931               & 0.2924               & 0.2892               & 0.0358                \\ 
\cline{1-8}\cline{10-17}
\textbf{landsat}         & 0.4716               & 0.4677               & 0.4854               & 0.4962               & 0.5089               & 0.5172               & 0.0457               &                      & \textbf{cardio}          & 0.4841               & 0.501                & 0.5083               & 0.5071               & 0.5125               & 0.5153               & 0.0312                \\ 
\cline{1-8}\cline{10-17}
\textbf{InternetAds}     & 0.6988               & 0.705                & 0.7088               & 0.715                & 0.7243               & 0.7348               & 0.0359               &                      & \textbf{skin}            & 0.2619               & 0.2597               & 0.276                & 0.2801               & 0.2864               & 0.2925               & 0.0306                \\ 
\cline{1-8}\cline{10-17}
\textbf{agnews\_1}       & 0.5995               & 0.6258               & 0.6272               & 0.6305               & 0.6324               & 0.6327               & 0.0332               &                      & \textbf{Stamps}          & 0.3182               & 0.3379               & 0.3457               & 0.351                & 0.3486               & 0.3468               & 0.0286                \\ 
\cmidrule[\heavyrulewidth]{1-8}\cmidrule[\heavyrulewidth]{10-17}
\multicolumn{1}{l}{}     & \multicolumn{1}{l}{} & \multicolumn{1}{l}{} & \multicolumn{1}{l}{} & \multicolumn{1}{l}{} & \multicolumn{1}{l}{} & \multicolumn{1}{l}{} & \multicolumn{1}{l}{} & \multicolumn{1}{l}{} & \multicolumn{1}{l}{}     & \multicolumn{1}{l}{} & \multicolumn{1}{l}{} & \multicolumn{1}{l}{} & \multicolumn{1}{l}{} & \multicolumn{1}{l}{} & \multicolumn{1}{l}{} & \multicolumn{1}{l}{}  \\ 
\cmidrule[\heavyrulewidth]{1-8}\cmidrule[\heavyrulewidth]{10-17}
\multicolumn{8}{c}{\textbf{ Student's improvement compared to Teacher (LOF) in terms of AUCROC}}                                                                                          &                      & \multicolumn{8}{c}{\textbf{Student's improvement compared to Teacher (LOF) in terms of AP}}                                                                                                \\ 
\cmidrule{1-8}\cmidrule{10-17}
\textbf{Datasets}        & \textbf{Teacher}     & \textbf{iter 2}      & \textbf{iter 4}      & \textbf{iter 6}      & \textbf{iter 8}      & \textbf{iter 10}     & \textbf{Improvement} &                      & \textbf{Datasets}        & \textbf{Teacher}     & \textbf{iter 2}      & \textbf{iter 4}      & \textbf{iter 6}      & \textbf{iter 8}      & \textbf{iter 10}     & \textbf{Improvement}  \\ 
\cmidrule{1-8}\cmidrule{10-17}
\textbf{http}            & 0.3685               & 1                    & 1                    & 1                    & 1                    & 1                    & 0.6315               &                      & \textbf{http}            & 0.0603               & 1                    & 1                    & 1                    & 1                    & 1                    & 0.9397                \\ 
\cline{1-8}\cline{10-17}
\textbf{shuttle}         & 0.4886               & 0.9199               & 0.9244               & 0.9691               & 0.9537               & 0.9525               & 0.4638               &                      & \textbf{shuttle}         & 0.0958               & 0.6814               & 0.7598               & 0.873                & 0.7902               & 0.7882               & 0.6924                \\ 
\cline{1-8}\cline{10-17}
\textbf{satimage-2}      & 0.4702               & 0.5677               & 0.6909               & 0.7618               & 0.8402               & 0.9146               & 0.4444               &                      & \textbf{optdigits}       & 0.0732               & 0.1114               & 0.1825               & 0.2627               & 0.3593               & 0.4551               & 0.3819                \\ 
\cline{1-8}\cline{10-17}
\textbf{optdigits}       & 0.5819               & 0.8488               & 0.8884               & 0.9128               & 0.9318               & 0.9438               & 0.3619               &                      & \textbf{satellite}       & 0.3746               & 0.6268               & 0.675                & 0.6887               & 0.7047               & 0.7117               & 0.3371                \\ 
\cline{1-8}\cline{10-17}
\textbf{musk}            & 0.4586               & 0.5008               & 0.5584               & 0.6137               & 0.6848               & 0.7528               & 0.2942               &                      & \textbf{WDBC}            & 0.1026               & 0.1757               & 0.2627               & 0.3202               & 0.3604               & 0.3754               & 0.2727                \\ 
\cline{1-8}\cline{10-17}
\textbf{satellite}       & 0.5523               & 0.7405               & 0.7655               & 0.7749               & 0.7868               & 0.7902               & 0.238                &                      & \textbf{FashionMNIST\_7} & 0.2485               & 0.3013               & 0.3345               & 0.3796               & 0.4325               & 0.4875               & 0.239                 \\ 
\cline{1-8}\cline{10-17}
\textbf{speech}          & 0.5035               & 0.6552               & 0.6823               & 0.7019               & 0.7115               & 0.7182               & 0.2147               &                      & \textbf{FashionMNIST\_1} & 0.1679               & 0.213                & 0.2372               & 0.2771               & 0.3291               & 0.3943               & 0.2263                \\ 
\cline{1-8}\cline{10-17}
\textbf{FashionMNIST\_5} & 0.6806               & 0.7116               & 0.7807               & 0.8211               & 0.8572               & 0.8847               & 0.2041               &                      & \textbf{FashionMNIST\_8} & 0.1246               & 0.1602               & 0.1917               & 0.2374               & 0.2996               & 0.3365               & 0.2119                \\ 
\cline{1-8}\cline{10-17}
\textbf{FashionMNIST\_1} & 0.6669               & 0.7405               & 0.7768               & 0.8083               & 0.833                & 0.8566               & 0.1897               &                      & \textbf{FashionMNIST\_5} & 0.1936               & 0.2157               & 0.2422               & 0.2776               & 0.3292               & 0.3971               & 0.2035                \\ 
\cline{1-8}\cline{10-17}
\textbf{landsat}         & 0.5436               & 0.704                & 0.7161               & 0.713                & 0.713                & 0.7096               & 0.166                &                      & \textbf{smtp}            & 0.0526               & 0.0556               & 0.3333               & 0.3333               & 0.25                 & 0.25                 & 0.1974                \\ 
\cmidrule[\heavyrulewidth]{1-8}\cmidrule[\heavyrulewidth]{10-17}
\multicolumn{1}{l}{}     & \multicolumn{1}{l}{} & \multicolumn{1}{l}{} & \multicolumn{1}{l}{} & \multicolumn{1}{l}{} & \multicolumn{1}{l}{} & \multicolumn{1}{l}{} & \multicolumn{1}{l}{} & \multicolumn{1}{l}{} & \multicolumn{1}{l}{}     & \multicolumn{1}{l}{} & \multicolumn{1}{l}{} & \multicolumn{1}{l}{} & \multicolumn{1}{l}{} & \multicolumn{1}{l}{} & \multicolumn{1}{l}{} & \multicolumn{1}{l}{}  \\ 
\cmidrule[\heavyrulewidth]{1-8}\cmidrule[\heavyrulewidth]{10-17}
\multicolumn{8}{c}{\textbf{ Student's improvement compared to Teacher (K-NN) in terms of AUCROC}}                                                                                         &                      & \multicolumn{8}{c}{\textbf{ Student's improvement compared to Teacher (K-NN) in terms of AP}}                                                                                              \\ 
\cmidrule{1-8}\cmidrule{10-17}
\textbf{Datasets}        & \textbf{Teacher}     & \textbf{iter 2}      & \textbf{iter 4}      & \textbf{iter 6}      & \textbf{iter 8}      & \textbf{iter 10}     & \textbf{Improvement} &                      & \textbf{Datasets}        & \textbf{Teacher}     & \textbf{iter 2}      & \textbf{iter 4}      & \textbf{iter 6}      & \textbf{iter 8}      & \textbf{iter 10}     & \textbf{Improvement}  \\ 
\cmidrule{1-8}\cmidrule{10-17}
\textbf{Stamps}          & 0.6587               & 0.773                & 0.8458               & 0.8863               & 0.8876               & 0.8851               & 0.2264               &                      & \textbf{shuttle}         & 0.1558               & 0.9055               & 0.9203               & 0.8229               & 0.7425               & 0.7379               & 0.5822                \\ 
\cline{1-8}\cline{10-17}
\textbf{SpamBase}        & 0.5086               & 0.6249               & 0.6675               & 0.692                & 0.7087               & 0.7119               & 0.2033               &                      & \textbf{satimage-2}      & 0.3294               & 0.4703               & 0.5803               & 0.6749               & 0.8082               & 0.8873               & 0.5579                \\ 
\cline{1-8}\cline{10-17}
\textbf{pendigits}       & 0.7133               & 0.8409               & 0.8484               & 0.8691               & 0.8861               & 0.9047               & 0.1914               &                      & \textbf{satellite}       & 0.5041               & 0.7098               & 0.7306               & 0.7448               & 0.7609               & 0.7683               & 0.2642                \\ 
\cline{1-8}\cline{10-17}
\textbf{musk}            & 0.6845               & 0.775                & 0.7961               & 0.8153               & 0.8377               & 0.8551               & 0.1706               &                      & \textbf{SpamBase}        & 0.3967               & 0.4643               & 0.5138               & 0.5479               & 0.5746               & 0.5815               & 0.1848                \\ 
\cline{1-8}\cline{10-17}
\textbf{shuttle}         & 0.6618               & 0.9908               & 0.9903               & 0.9365               & 0.8425               & 0.8134               & 0.1516               &                      & \textbf{WPBC}            & 0.232                & 0.2343               & 0.2788               & 0.3481               & 0.3952               & 0.4123               & 0.1803                \\ 
\cline{1-8}\cline{10-17}
\textbf{speech}          & 0.4791               & 0.5861               & 0.6065               & 0.6213               & 0.626                & 0.6289               & 0.1498               &                      & \textbf{Stamps}          & 0.1598               & 0.1868               & 0.2292               & 0.2873               & 0.322                & 0.3343               & 0.1745                \\ 
\cline{1-8}\cline{10-17}
\textbf{WPBC}            & 0.4643               & 0.4833               & 0.5247               & 0.5555               & 0.589                & 0.6088               & 0.1445               &                      & \textbf{musk}            & 0.0897               & 0.0805               & 0.0969               & 0.132                & 0.2204               & 0.253                & 0.1633                \\ 
\cline{1-8}\cline{10-17}
\textbf{satellite}       & 0.6536               & 0.7617               & 0.7724               & 0.7788               & 0.7889               & 0.7932               & 0.1396               &                      & \textbf{wine}            & 0.0789               & 0.1071               & 0.1403               & 0.2368               & 0.244                & 0.2422               & 0.1633                \\ 
\cline{1-8}\cline{10-17}
\textbf{WBC}             & 0.8503               & 0.9611               & 0.9688               & 0.9756               & 0.9819               & 0.9736               & 0.1234               &                      & \textbf{landsat}         & 0.2511               & 0.3578               & 0.3689               & 0.3738               & 0.38                 & 0.3839               & 0.1328                \\ 
\cline{1-8}\cline{10-17}
\textbf{WDBC}            & 0.7211               & 0.7883               & 0.8263               & 0.8357               & 0.8406               & 0.839                & 0.1179               &                      & \textbf{annthyroid}      & 0.1742               & 0.1874               & 0.2024               & 0.2207               & 0.251                & 0.3014               & 0.1272                \\ 
\cmidrule[\heavyrulewidth]{1-8}\cmidrule[\heavyrulewidth]{10-17}
\multicolumn{1}{l}{}     & \multicolumn{1}{l}{} & \multicolumn{1}{l}{} & \multicolumn{1}{l}{} & \multicolumn{1}{l}{} & \multicolumn{1}{l}{} & \multicolumn{1}{l}{} & \multicolumn{1}{l}{} & \multicolumn{1}{l}{} & \multicolumn{1}{l}{}     & \multicolumn{1}{l}{} & \multicolumn{1}{l}{} & \multicolumn{1}{l}{} & \multicolumn{1}{l}{} & \multicolumn{1}{l}{} & \multicolumn{1}{l}{} & \multicolumn{1}{l}{}  \\ 
\cmidrule[\heavyrulewidth]{1-8}\cmidrule[\heavyrulewidth]{10-17}
\multicolumn{8}{c}{\textbf{ Student's improvement compared to Teacher (OCSVM) in terms of AUCROC}}                                                                                        &                      & \multicolumn{8}{c}{\textbf{ Student's improvement compared to Teacher (OCSVM) in terms of AP}}                                                                                             \\ 
\cmidrule{1-8}\cmidrule{10-17}
\textbf{Datasets}        & \textbf{Teacher}     & \textbf{iter 2}      & \textbf{iter 4}      & \textbf{iter 6}      & \textbf{iter 8}      & \textbf{iter 10}     & \textbf{Improvement} &                      & \textbf{Datasets}        & \textbf{Teacher}     & \textbf{iter 2}      & \textbf{iter 4}      & \textbf{iter 6}      & \textbf{iter 8}      & \textbf{iter 10}     & \textbf{Improvement}  \\ 
\cmidrule{1-8}\cmidrule{10-17}
\textbf{speech}          & 0.4634               & 0.6196               & 0.6152               & 0.6207               & 0.6242               & 0.6264               & 0.163                &                      & \textbf{wine}            & 0.1776               & 0.18                 & 0.21                 & 0.2663               & 0.3382               & 0.4178               & 0.2402                \\ 
\cline{1-8}\cline{10-17}
\textbf{agnews\_1}       & 0.5654               & 0.6128               & 0.6408               & 0.6697               & 0.6878               & 0.7026               & 0.1372               &                      & \textbf{pendigits}       & 0.2283               & 0.3174               & 0.3397               & 0.3461               & 0.3625               & 0.3544               & 0.1262                \\ 
\cline{1-8}\cline{10-17}
\textbf{Wilt}            & 0.37                 & 0.3282               & 0.3038               & 0.3541               & 0.4366               & 0.4995               & 0.1295               &                      & \textbf{thyroid}         & 0.1352               & 0.1456               & 0.1613               & 0.1793               & 0.2047               & 0.2395               & 0.1044                \\ 
\cline{1-8}\cline{10-17}
\textbf{annthyroid}      & 0.5969               & 0.6216               & 0.6382               & 0.6623               & 0.684                & 0.7108               & 0.1139               &                      & \textbf{annthyroid}      & 0.1294               & 0.138                & 0.1481               & 0.1645               & 0.1809               & 0.2046               & 0.0751                \\ 
\cline{1-8}\cline{10-17}
\textbf{vowels}          & 0.5529               & 0.5783               & 0.6106               & 0.6213               & 0.6468               & 0.6612               & 0.1083               &                      & \textbf{vowels}          & 0.0508               & 0.0476               & 0.0538               & 0.0591               & 0.0958               & 0.1243               & 0.0735                \\ 
\cline{1-8}\cline{10-17}
\textbf{SpamBase}        & 0.5109               & 0.5244               & 0.5558               & 0.5827               & 0.598                & 0.604                & 0.0931               &                      & \textbf{SpamBase}        & 0.3862               & 0.3893               & 0.4079               & 0.4306               & 0.447                & 0.4578               & 0.0716                \\ 
\cline{1-8}\cline{10-17}
\textbf{landsat}         & 0.3631               & 0.3932               & 0.4034               & 0.4086               & 0.4175               & 0.4208               & 0.0577               &                      & \textbf{cardio}          & 0.5858               & 0.6321               & 0.6257               & 0.6198               & 0.6261               & 0.6251               & 0.0393                \\ 
\cline{1-8}\cline{10-17}
\textbf{satellite}       & 0.5944               & 0.618                & 0.6249               & 0.6301               & 0.6368               & 0.6421               & 0.0477               &                      & \textbf{PageBlocks}      & 0.4882               & 0.5087               & 0.513                & 0.5265               & 0.5222               & 0.5228               & 0.0346                \\ 
\cline{1-8}\cline{10-17}
\textbf{wine}            & 0.6359               & 0.6462               & 0.6583               & 0.6619               & 0.6733               & 0.6789               & 0.0431               &                      & \textbf{satellite}       & 0.5814               & 0.5913               & 0.5975               & 0.6031               & 0.6097               & 0.6142               & 0.0328                \\ 
\cline{1-8}\cline{10-17}
\textbf{agnews\_0}       & 0.5156               & 0.5159               & 0.5184               & 0.529                & 0.5429               & 0.5579               & 0.0423               &                      & \textbf{FashionMNIST\_7} & 0.7066               & 0.7124               & 0.7172               & 0.7224               & 0.7285               & 0.7385               & 0.0319                \\
\cmidrule[\heavyrulewidth]{1-8}\cmidrule[\heavyrulewidth]{10-17}
\end{tabular}}
\end{table*}
